# Supplementary material for: Pruning Neural Networks at Initialization: Why are We Missing the Mark?
Source: arXiv:2009.08576 source file (2021-03-21)
Supplement: Supplementary file 1 [file ablations-at-init.tex]

\section{Ablations for OMP, SNIP, and GraSP at Initialization}
\label{app:ablations}

In this Appendix, we conduct several ablation studies on one-shot magnitude pruning (OMP), SNIP, and GraSP when applied at initialization to the neural networks from the GraSP paper (Appendix \ref{app:grasp}, Table \ref{tab:grasp-networks}) at the sparsities in the GraSP paper.
Our goal is to understand the specificity of the scores issued by these heuristics and the extent to which the heuristics behave in accordance with the justifications provided by \citet{lee2019snip} and \citet{wang2020picking}.

For each technique, we perform the following experiments with the scores $s$ assigned to the weights by the technique.
\begin{itemize}
    \item The standard version of the technique (marked with a * in each table).
    \item Randomly shuffling the scores within each layer before pruning. This experiment assesses whether the technique is learning which specific parameters to prune or the layerwise proportions by which to prune the network.
    \item Randomly reinitializing the network. This experiment assesses whether the technique is specific to the initial values of the parameters.
    \item Pruning the parameters that the technique considers least important (e.g., pruning parameters with the highest scores if the technique typically prunes the parameters with the lowest scores). This experiment assesses the validity of the mapping between scores and importance.
\end{itemize}

\subsection{One-Shot Magnitude Pruning}

Table \ref{tab:ablation-omp} below conducts the ablations for one-shot magnitude pruning at initialization.
It is possible to randomly shuffle the pruning masks found at initialization and to randomly reinitialize the pruned network without substantial change in accuracy.
This means that, at initialization, OMP is identifying only layerwise proportions in which to prune the network.
It is not identifying the specific sparse structure within each pruned layer or the specific initial weights to retain.
OMP correctly determines that high-magnitude parameters are more important to final accuracy than low-high-magnitude parameters, but it is possible that pruning high-magnitude weights simply selects poor layerwise proportions in which to prune the network.

\begin{table}[h]
%\resizebox{\textwidth}{!}{%
\centering
\small
\begin{tabular}{l | c c c c c}
    \toprule
    Name & Sparsity & Lowest $s$* & Lowest $s$ (Shuffled) & Lowest $s$ (Reinit) & Highest $s$ \\ \midrule
    \multirow{3}{*}{VGG-19}
	 & $90\%$ & $92.8\%$ & $92.8\%$ $(+0.0)$ & $93.0\%$ $(+0.2)$ & $88.4\%$ $(-4.4)$ \\
	 & $95\%$ & $92.4\%$ & $92.4\%$ $(+0.0)$ & $92.4\%$ $(+0.0)$ & $85.3\%$ $(-7.1)$ \\
	 & $98\%$ & $91.6\%$ & $91.6\%$ $(+0.0)$ & $91.7\%$ $(+0.1)$ & $10.0\%$ $(-81.6)$ \\
	 \midrule
    \multirow{3}{*}{WRN-32-2}
	 & $90\%$ & $92.4\%$ & $92.5\%$ $(+0.1)$ & $92.6\%$ $(+0.2)$ & $90.7\%$ $(-1.7)$ \\
	 & $95\%$ & $91.0\%$ & $91.3\%$ $(+0.3)$ & $91.3\%$ $(+0.3)$ & $83.2\%$ $(-7.8)$ \\
	 & $98\%$ & $88.0\%$ & $88.4\%$ $(+0.4)$ & $88.3\%$ $(+0.3)$ & $50.9\%$ $(-37.1)$ \\
	 \midrule
    \multirow{3}{*}{ResNet-50}
	 & $60\%$ & $74.1\%$ & $74.2\%$ $(+0.1)$ & $74.1\%$ $(+0.0)$ & $72.0\%$ $(-2.1)$ \\
	 & $80\%$ & $71.0\%$ & $71.3\%$ $(+0.3)$ & $47.5\%$ $(-23.5)$ & $67.8\%$ $(-3.2)$ \\
	 & $90\%$ & $65.5\%$ & $65.9\%$ $(+0.4)$ & $65.8\%$ $(+0.3)$ & $62.3\%$ $(-3.2)$ \\    
	 \bottomrule
\end{tabular}
%}
\label{tab:ablation-omp}
\caption{Accuracies for the ablation studies for one-shot magnitude pruning (OMP) at initialization.
Scores issued by OMP are represented by $s$. 
The standard version of OMP is marked with *.
Numbers in parentheses are the change in accuracy from the standard version.}
\end{table}

\subsection{SNIP}

Table \ref{tab:ablation-snip} below conducts the ablations for SNIP at initialization.
The analysis from OMP also applies to SNIP.
It is possible to randomly shuffle the pruning masks found at initialization and to randomly reinitialize the pruned network without substantial change in accuracy.
This means that, at initialization, SNIP is identifying only layerwise proportions in which to prune the network.
It is not identifying the specific sparse structure within each pruned layer or the specific initial weights to retain.
SNIP correctly determines that high-scoring parameters are more important to final accuracy than low-scoring parameters, but it is possible that pruning high-scoring weights simply selects poor layerwise proportions in which to prune the network.

\begin{table}[h]
%\resizebox{\textwidth}{!}{%
\centering
\small
\begin{tabular}{l | c c c c c}
    \toprule
    Name & Sparsity & Lowest $s$* & Lowest $s$ (Shuffled) & Lowest $s$ (Reinit) & Highest $s$ \\ \midrule
    \multirow{3}{*}{VGG-19}
	 & $90\%$ & $93.5\%$ & $93.3\%$ $(-0.2)$ & $93.4\%$ $(-0.1)$ & $51.6\%$ $(-41.9)$ \\
	 & $95\%$ & $93.4\%$ & $93.2\%$ $(-0.2)$ & $93.1\%$ $(-0.3)$ & $10.0\%$ $(-83.4)$ \\
	 & $98\%$ & $42.7\%$ & $55.8\%$ $(+13.1)$ & $40.4\%$ $(-2.3)$ & $10.0\%$ $(-32.7)$ \\
	 \midrule
    \multirow{3}{*}{WRN-32-2}
	 & $90\%$ & $92.5\%$ & $92.5\%$ $(+0.0)$ & $92.3\%$ $(-0.2)$ & $11.8\%$ $(-80.7)$ \\
	 & $95\%$ & $91.0\%$ & $91.1\%$ $(+0.1)$ & $90.7\%$ $(-0.3)$ & $10.0\%$ $(-81.0)$ \\
	 & $98\%$ & $87.7\%$ & $88.0\%$ $(+0.3)$ & $87.7\%$ $(+0.0)$ & $11.7\%$ $(-76.0)$ \\
	 \midrule
    \multirow{3}{*}{ResNet-50}
	 & $60\%$ & $74.2\%$ & $74.2\%$ $(+0.0)$ & $74.1\%$ $(-0.1)$ & $65.6\%$ $(-8.6)$ \\
	 & $80\%$ & $71.1\%$ & $71.2\%$ $(+0.1)$ & $71.2\%$ $(+0.1)$ & $19.7\%$ $(-51.4)$ \\
	 & $90\%$ & $64.7\%$ & $66.4\%$ $(+1.7)$ & $65.7\%$ $(+1.0)$ & $0.1\%$ $(-64.6)$ \\
	 \bottomrule
\end{tabular}
%}
\label{tab:ablation-snip}
\caption{Accuracies for the ablation studies for SNIP at initialization.
Scores issued by SNIP are represented by $s$. 
The standard version of SNIP is marked with *.
Numbers in parentheses are the change in accuracy from the standard version.}
\end{table}

\subsection{GraSP}

Table \ref{tab:ablation-grasp} below conducts the ablations for GraSP at initialization.
Like OMP and SNIP, it is possible to randomly shuffle the GraSP pruning masks found at initialization and to randomly reinitialize the pruned network without substantial change in accuracy.
This means that, at initialization, GraSP is identifying only layerwise proportions in which to prune the network.

Unlike OMP and SNIP, GraSP produces a signed score, where a positive score means removing a parameter improves gradient flow and a negative score means removing a parameter reduces gradient flow.
By the interpretation of \citet{wang2020picking}, it is beneficial to prune those parameters that most improve (or least reduce) gradient flow; that is, those parameters with the lowest scores are the most important.
However, the data in Table \ref{tab:ablation-grasp} does not support this interpretation: pruning parameters with the lowest scores does not affect accuracy.
In other words, it is just as effective to prune with the intention of destroying gradient flow (according to the GraSP scores) as it is to prune with the intention of ``preserving gradient flow.''

In light of these results, we attempted one further ablation: pruning scores with the lowest magnitudes.
Since it is equally effective to prune the lowest or highest scores, we hypothesized that the magnitude of the scores may also be a useful signal.
Indeed, we find that performance slightly improves when using the lowest magnitude scores in this way.
However, pruning the highest magnitude scores results in significant drops in accuracy.

We conclude that, although the GraSP scores do extract useful information from the network, the justification for the scores provided by \citet{wang2020picking} does not match the results in Table \ref{tab:ablation-grasp}.

\begin{table}[h]
\resizebox{\textwidth}{!}{%
\begin{tabular}{l | c c c c c c c}
    \toprule
    Name & Sparsity & Highest $s$* & Highest $s$ (Shuffled) & Highest $s$ (Reinit) & Lowest $s$ & Lowest $|s|$ & Highest $|s|$ \\ \midrule
    \multirow{3}{*}{VGG-19}
	 & $90\%$ & $92.8\%$ & $92.9\%$ $(+0.1)$ & $92.9\%$ $(+0.1)$ & $92.8\%$ $(+0.0)$ & $93.2\%$ $(+0.4)$ & $67.5\%$ $(-25.3)$ \\
	 & $95\%$ & $92.5\%$ & $92.5\%$ $(+0.0)$ & $92.6\%$ $(+0.1)$ & $92.4\%$ $(-0.1)$ & $92.9\%$ $(+0.4)$ & $37.0\%$ $(-55.5)$ \\
	 & $98\%$ & $91.9\%$ & $91.8\%$ $(-0.1)$ & $91.8\%$ $(-0.1)$ & $91.7\%$ $(-0.2)$ & $92.1\%$ $(+0.2)$ & $10.0\%$ $(-81.9)$ \\
	 \midrule
    \multirow{3}{*}{WRN-32-2}
	 & $90\%$ & $92.2\%$ & $92.2\%$ $(+0.0)$ & $92.2\%$ $(+0.0)$ & $92.2\%$ $(+0.0)$ & $92.4\%$ $(+0.2)$ & $31.3\%$ $(-60.9)$ \\
	 & $95\%$ & $90.9\%$ & $91.1\%$ $(+0.2)$ & $91.3\%$ $(+0.4)$ & $91.1\%$ $(+0.2)$ & $91.2\%$ $(+0.3)$ & $18.7\%$ $(-72.2)$ \\
	 & $98\%$ & $88.3\%$ & $88.5\%$ $(+0.2)$ & $88.4\%$ $(+0.1)$ & $88.4\%$ $(+0.1)$ & $88.3\%$ $(+0.0)$ & $11.6\%$ $(-76.7)$ \\
	 \midrule
    \multirow{3}{*}{ResNet-50}
	 & $60\%$ & $73.4\%$ & $73.6\%$ $(+0.2)$ & $73.6\%$ $(+0.2)$ & $73.3\%$ $(-0.1)$ & $74.1\%$ $(+0.7)$ & $69.7\%$ $(-3.7)$ \\
	 & $80\%$ & $71.0\%$ & $70.8\%$ $(-0.2)$ & $71.1\%$ $(+0.1)$ & $70.7\%$ $(-0.3)$ & $71.6\%$ $(+0.6)$ & $63.8\%$ $(-7.2)$ \\
	 & $90\%$ & $67.3\%$ & $67.3\%$ $(+0.0)$ & $67.2\%$ $(-0.1)$ & $66.8\%$ $(-0.5)$ & $67.8\%$ $(+0.5)$ & $52.2\%$ $(-15.1)$ \\
	 \bottomrule
\end{tabular}
}
\label{tab:ablation-grasp}
\caption{Accuracies for the ablation studies for GraSP at initialization.
Scores issued by GraSP are represented by $s$. 
The standard version of GraSP is marked with *.
Numbers in parentheses are the change in accuracy from the standard version.
This table includes an additional ablation where we prune parameters with the lowest-magnitude scores.}
\end{table}
