# Supplementary material for: Pruning Neural Networks at Initialization: Why are We Missing the Mark?
Source: arXiv:2009.08576 source file (2021-03-21)
Supplement: Supplementary file 2 [file concurrent.tex]

\section{Comparison to Concurrent Work}
\label{app:concurrent}

Concurrently and independently, \citet{su2020sanity} conducted shuffling ablations on SNIP and GraSP.
According to emails with the ICLR program chairs, ICLR ``follow[s] the NeurIPS policy of treating papers concurrent if they are published in the two months prior to our paper deadline.'' This means that we are ``not...responsible for comparing with papers published on or after Aug 2.'' The paper we discuss here was released on arXiv on Sep 22 and will not be published until NeurIPS occurs Dec 7, so it qualifies as concurrent work.
However, we include this comparison for the sake of rigor.\vspace{-1mm}

\textbf{Similarities in findings.} Our findings overlap with those of \citeauthor{su2020sanity} in the following ways:

\begin{itemize}[leftmargin=1em,itemsep=1pt,parsep=1pt,topsep=0pt,partopsep=0pt]
    \item We perform ablations to understand the information that pruning methods extract at initialization.
    \item We find that SNIP and GraSP maintain the same accuracy under the shuffling ablation.
    \item We show a ``zero-shot'' way to reach accuracy similar to SNIP and GraSP by selecting appropriate layer-wise pruning rates and pruning randomly.\footnote{While the ``zero-shot'' approach of \citeauthor{su2020sanity}~involves picking arbitrary per-layer pruning proportions based on depth, we find that we can simply use the proportions implicitly provided by the Kaiming variance-scaled initialization without additional work. We find this because we include magnitude pruning at initialization.}
\end{itemize}

\textbf{Differences in findings.} Our findings are distinct from those of \citeauthor{su2020sanity}~in the following ways:

\begin{itemize}[leftmargin=1em,itemsep=1pt,parsep=1pt,topsep=0pt,partopsep=0pt]
    \item In addition to SNIP and GraSP, we also show that these results hold for magnitude pruning, SynFlow, and iterative SNIP (Appendix \ref{app:iterative-snip}).
    \item We compare these methods at 14-18 sparsities (vs. 3 in \citeauthor{su2020sanity}) and include baselines (random pruning and magnitude after training).
          This allows us to reach the broader conclusions about the state of the art in pruning at initialization in Section \ref{sec:baselines}.
    \item We perform reinitialization\footnote{In their methodology, \citeauthor{su2020sanity}~mention an experiment where weights (but not masks) are shuffled within each layer in a manner similar to reinitialization. However, they do not perform this ablation on SNIP or GraSP.} and inversion ablations, and we show the practical value of ablations by using them to diagnose and improve GraSP (inversion) and SynFlow (neuron collapse).
    \item We show that the performance of the pruning methods improves only gradually if pruning occurs later in training, and we perform ablations on the pruning methods after training (Appendix \ref{app:ablations-after}).
\end{itemize}

\textbf{Differences in conclusions.}
These different findings lead us to different conclusions.
\citeauthor{su2020sanity}~conclude that the shuffling results ``cast[s] doubt on whether the[] individual connections in the pruned subnetwork [are] crucial'' and that ``the architecture of the pruned network may only have limited impact on the final performance.''\footnote{Although it is unclear in the paper, we presume \citeauthor{su2020sanity}~intend these claims to be specific to SNIP and GraSP rather than to apply to pruning in general (where there are known counterexamples, e.g., Appendix \ref{app:ablations-after}).}
We conclude more broadly that the ablations imply limitations inherent to these methods or to pruning at initialization.
We are able to draw this conclusion using the baseline of magnitude pruning after training, which (a) reaches higher accuracy and (b) is not robust to ablations.
This shows that there are indeed settings for which the pruned architecture matters and that there may be a connection between sensitivity to the ablations and accuracy.

\textbf{Differences in breadth.} Our findings are broader in the following ways:
\begin{itemize}[leftmargin=1em,itemsep=1pt,parsep=1pt,topsep=0pt,partopsep=0pt]
    \item We study more early pruning methods (SynFlow, magnitude, iterative SNIP).
    \item We include baselines (random, magnitude after training), neither of which are in \citeauthor{su2020sanity}\footnote{\citeauthor{su2020sanity}~include two experiments that they describe as lottery tickets. The first (which they call LT) involves rewinding to initialization, which is known to perform poorly on the networks that they study \citep{frankle2020lottery}. The second (which they call Learning Rate Rewinding after \citet{Renda2020Comparing}) is similar to our LTR baseline, although they do not specify the specific rewinding iterations that they use.}
    \item We include experiments on ResNet-50 on ImageNet, larger-scale than the CIFAR-10 and TinyImageNet experiments in \citeauthor{su2020sanity}
    \item We conduct our main experiments at between 14 and 18 different sparsities. \citeauthor{su2020sanity}~conduct ablations at five sparsities and compare between methods at three sparsities.
\end{itemize}
