# Supplementary material for: Pruning Neural Networks at Initialization: Why are We Missing the Mark?
Source: arXiv:2009.08576 source file (2021-03-21)
Supplement: Supplementary file 3 [file concurrent-work-policy.tex]

\section{ICLR 2021 Concurrent Work Policy}
\label{app:concurrent-work-policy}

According to correspondence with the ICLR 2021 program chairs:

\emph{We will follow the NeurIPS policy of treating papers concurrent if they are published in the two months prior to our paper deadline. So you will not be responsible for comparing with papers published on or after Aug 2.}
