# Supplementary material for: Pruning Neural Networks at Initialization: Why are We Missing the Mark?
Source: arXiv:2009.08576 source file (2021-03-21)
Supplement: Supplementary file 4 [file tables.tex]

\section{Tables of Numbers}

To facilitate easier comparisons and replication in the future, we have included tables of all of the numbers that went into our plots.
All numbers are mean $\pm$ stddev over five replicates (CIFAR-10) or three replicates (TinyImageNet and ImageNet).
